# Supplementary material for: Compactification of Determinant Expansions via Transcorrelation
Source: arXiv:2405.02640 ancillary file (2024-05-04)
Supplement: Supplementary file 1 [file si.pdf]

# Compactification of CI Expansions via Transcorrelation

Abdallah Ammar,[1, a)] Anthony Scemama,[1, b)] Pierre-François Loos,[1, c)] and Emmanuel Giner[2, d)]
[1)] *Laboratoire de Chimie et Physique Quantiques (UMR 5626), Université de Toulouse, CNRS, UPS, France*
[2)] *Laboratoire de Chimie Théorique, Sorbonne Université and CNRS, F-75005 Paris, France*

## I. MOLECULAR GEOMETRIES

Molecular coordinates for $Li_2$ (in Angstroms):

| | | | |
|---|---|---|---|
| Li | 0.0000 | 0.0000 | − 1.3365 |
| Li | 0.0000 | 0.0000 | + 1.3365 |

Molecular coordinates for $Be_2$ (in Angstroms):

| | | | |
|---|---|---|---|
| Be | 0.0000 | 0.0000 | 0.0000 |
| Be | 0.0000 | 0.0000 | 2.4450 |

Molecular coordinates for $H_2O$ (in Angstroms):

| | | | |
|---|---|---|---|
| O | 0.0000 | + 0.0000 | − 0.0699 |
| H | 0.0000 | + 0.7575 | + 0.5184 |
| H | 0.0000 | − 0.7575 | + 0.5184 |

Molecular coordinates for $NH_3$ (in Angstroms):

| | | | |
|---|---|---|---|
| N | + 0.0678 | + 0.0000 | + 0.0000 |
| H | − 0.3138 | + 0.4688 | − 0.8119 |
| H | − 0.3138 | − 0.9375 | + 0.0000 |
| H | − 0.3138 | + 0.4688 | + 0.8119 |

Molecular coordinates for $CH_4$ (in Angstroms):

| | | | |
|---|---|---|---|
| C | + 0.0000 | + 0.0000 | + 0.0000 |
| H | + 1.0879 | + 0.0000 | + 0.0000 |
| H | − 0.3626 | + 1.0257 | + 0.0000 |
| H | − 0.3626 | − 0.5128 | − 0.8883 |
| H | − 0.3626 | − 0.5128 | + 0.8883 |

Molecular coordinates for $H_2CO$ (in Angstroms):

| | | | |
|---|---|---|---|
| C | 0.0000 | + 0.0000 | − 0.6030 |
| O | 0.0000 | + 0.0000 | + 0.6054 |
| H | 0.0000 | + 0.9347 | − 1.1822 |
| H | 0.0000 | − 0.9347 | − 1.1822 |

[a)]Electronic mail: aammar@irsamc.ups-tlse.fr
[b)]Electronic mail: scemama@irsamc.ups-tlse.fr
[c)]Electronic mail: loos@irsamc.ups-tlse.fr
[d)]Electronic mail: emmanuel.giner@lct.jussieu.fr

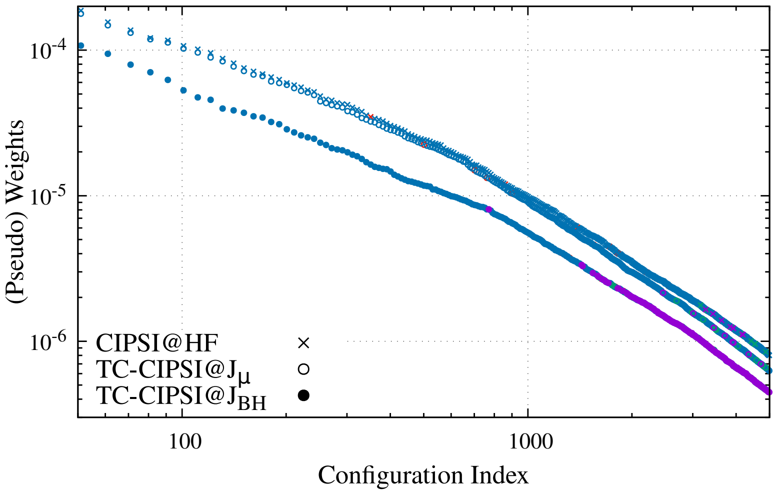


FIG. 1. $H_2O$@cc-pVTZ: Weights ($c_I^2$) of the CIPSI wave function and pseudo-weights ($|\tilde{c}_I c_I|$) of the TC-CIPSI wave function using two types of correlation factors: the 9-parameter correlation factor of Boys and Handy obtained in Ref. 1 (labelled as TC-CIPSI@$J_{BH}$) and the one-parameter correlation factor introduced in Ref. 2 (labelled as TC-CIPSI@$J_\mu$). The excitation degree of each determinant with respect to the mean-field reference determinant is indicated by the following color code: red, blue, green, and purple for single, double, triple, and quadruple excitations, respectively.

## II. RESULTS

In Fig. 1 we report the weights of the CIPSI wave function and pseudo weights of the TC-CIPSI wave function in the case of the $H_2O$ molecule in the cc-pVTZ basis set. With respect to Fig. 2 of the manuscript where calculations are performed using the nine-parameter correlation factor of Ref. 1, we also report here calculations performed with the rather simple one-parameter correlation factor introduced in Ref. 2.

In Table I, we present a comparison of the convergence between CIPSI and TC-CIPSI, based on the second-order energy criterion. The table displays the number of determinants required to achieve second-order energies of $1.5\,\text{m}E_\text{h}$, $3.0\,\text{m}E_\text{h}$, $7.5\,\text{m}E_\text{h}$, $15.0\,\text{m}E_\text{h}$, and $30.0\,\text{m}E_\text{h}$ for the $Li_2$, $H_2O$, $NH_3$, $CH_4$, and $H_2CO$ molecules across various basis sets. It is evident that TC-CIPSI converges much more rapidly than CIPSI, with the number of determinants needed being reduced by a factor ranging between 2 and 42 in cc-pVDZ, 5 and 121 in cc-pVTZ, and 6 and 1709 in cc-pVQZ.

In Table II, we provide a comparison of the number of determinants required to achieve convergence over extrapolation for these molecules across the various basis sets considered. With the exception of the calculation on $H_2CO$ in the cc-pVDZ basis set, where convergence is achieved with a similar number of determinants, we observed that TC-CIPSI converges with a smaller number of determinants compared to CIPSI, typically by a factor ranging between 3 and 7.

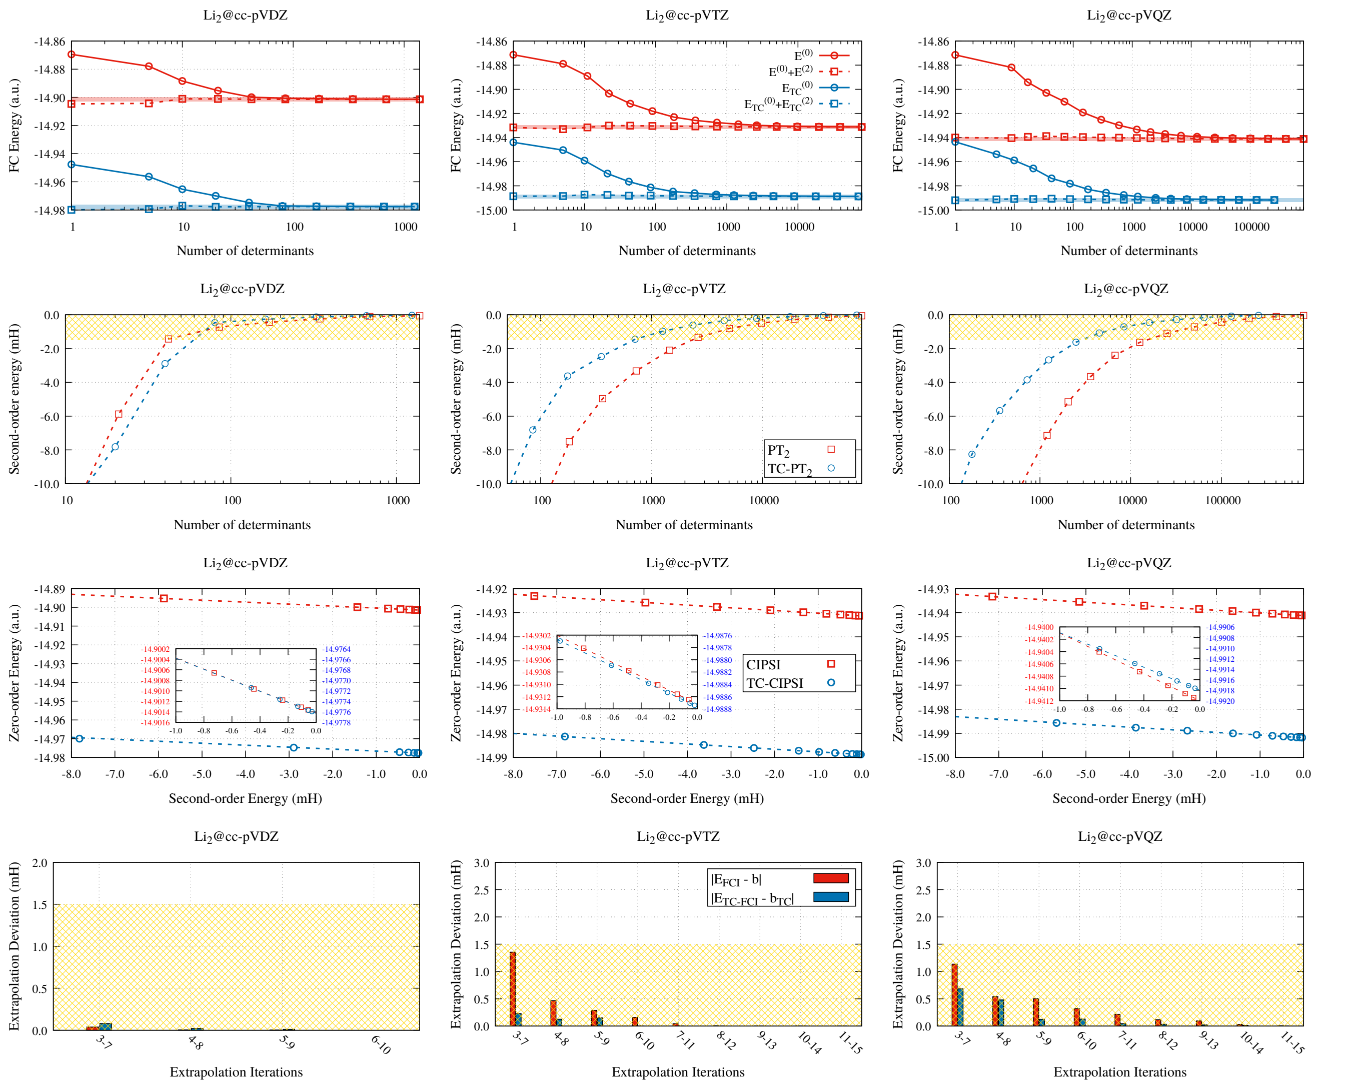


FIG. 2. Convergence analysis of frozen-core calculations for $Li_2$ molecule using different basis sets. Each row represents a different aspect of the convergence analysis, with three panels corresponding to different basis sets: cc-pVDZ (left), cc-pVTZ (middle), and cc-pVQZ (right).

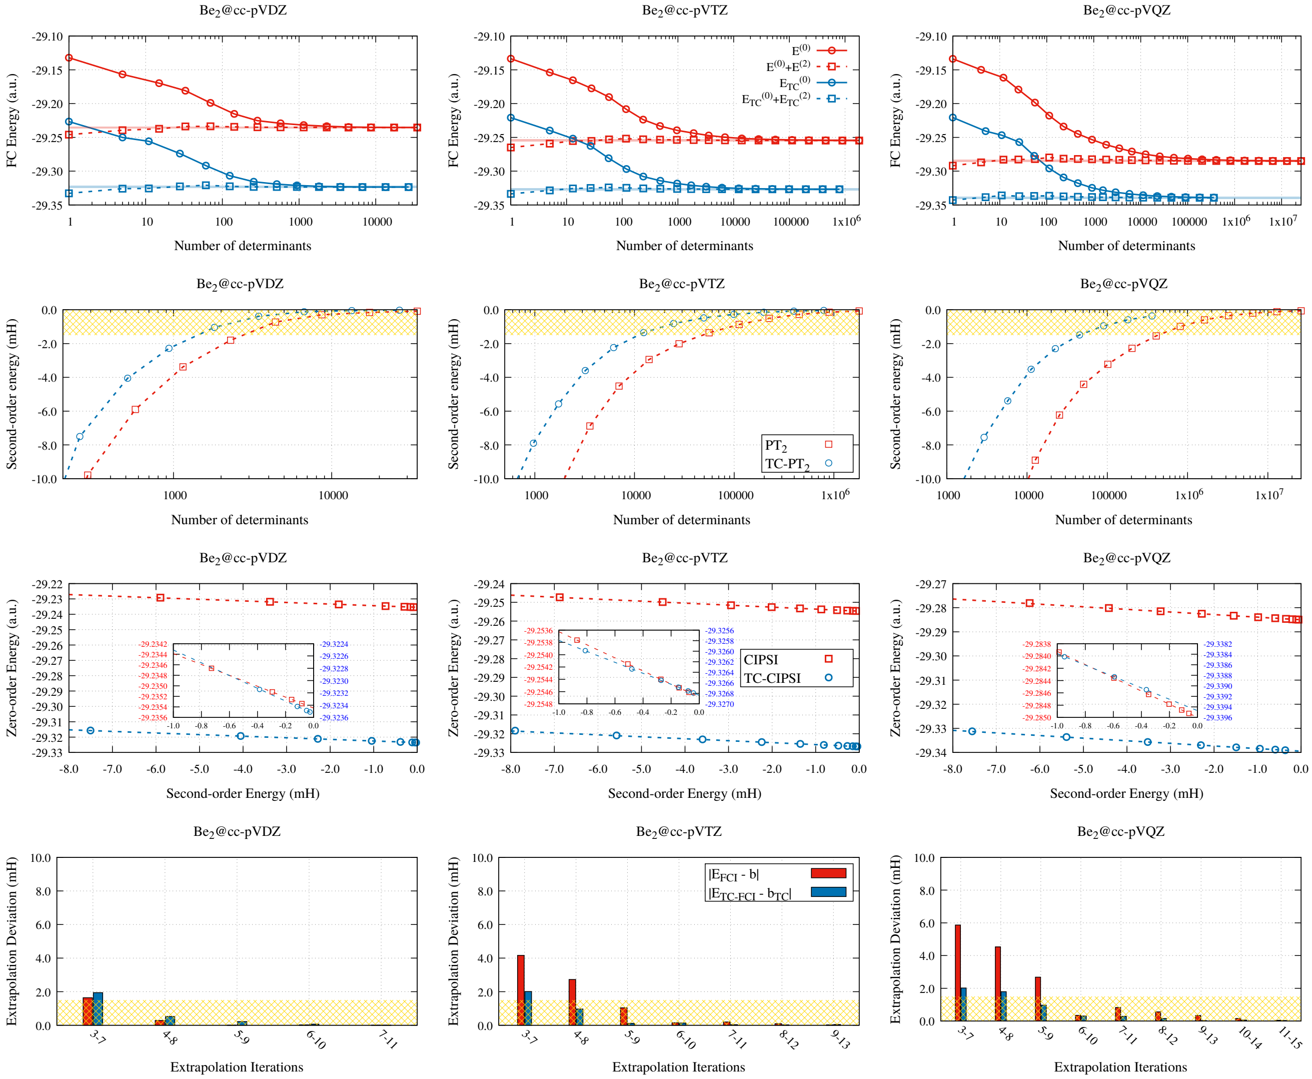


FIG. 3. Convergence analysis of frozen-core calculations for $Be_2$ molecule using different basis sets. Each row represents a different aspect of the convergence analysis, with three panels corresponding to different basis sets: cc-pVDZ (left), cc-pVTZ (middle), and cc-pVQZ (right).

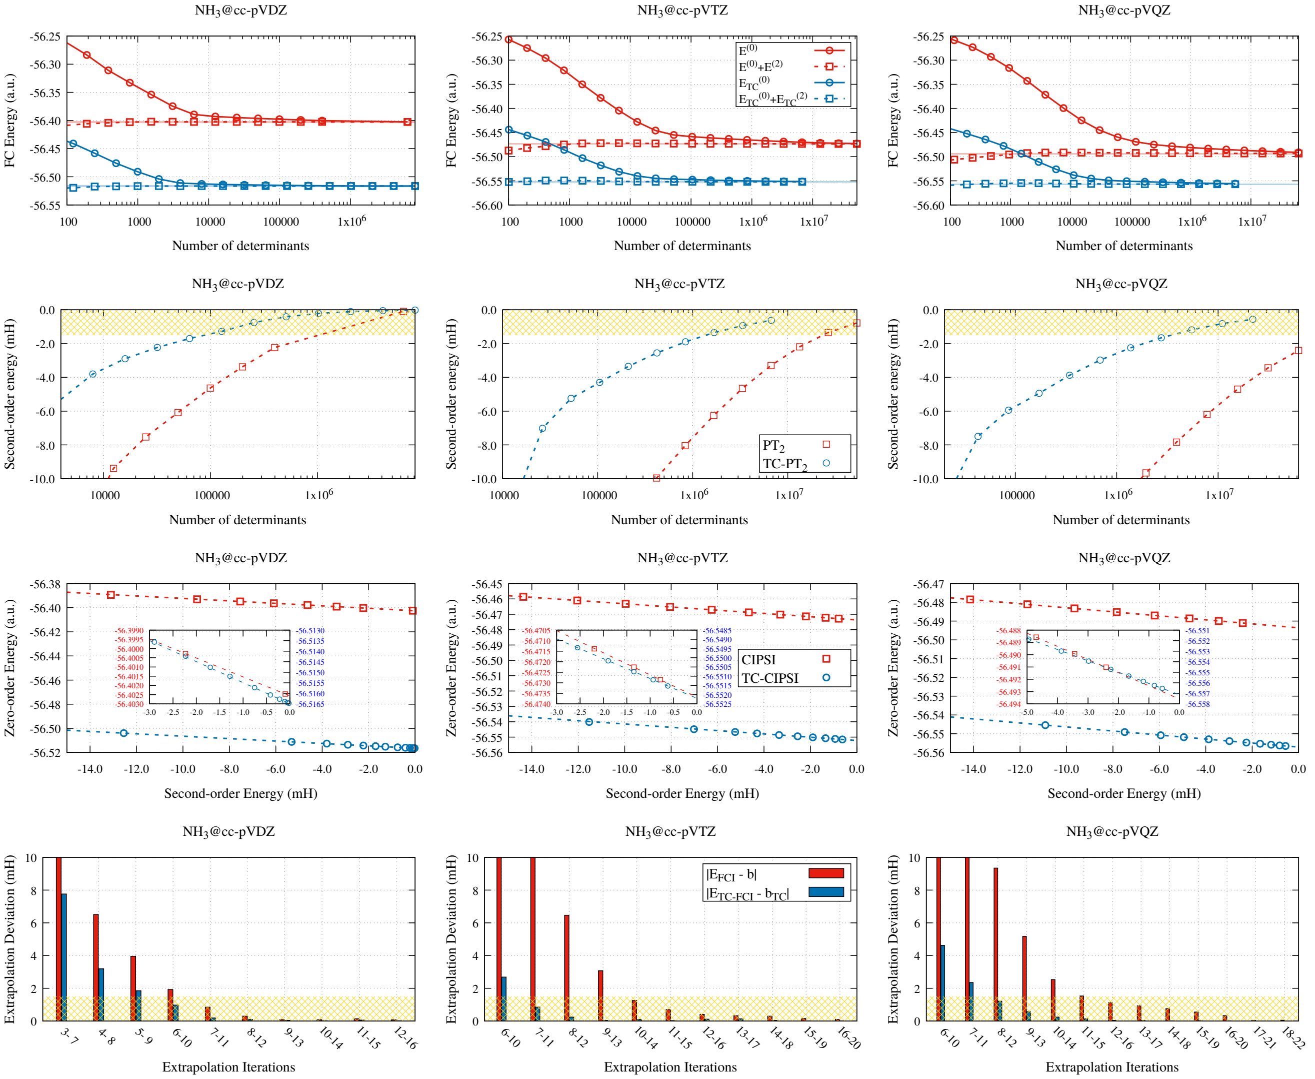


FIG. 4. Convergence analysis of frozen-core calculations for $NH_3$ molecule using different basis sets. Each row represents a different aspect of the convergence analysis, with three panels corresponding to different basis sets: cc-pVDZ (left), cc-pVTZ (middle), and cc-pVQZ (right).

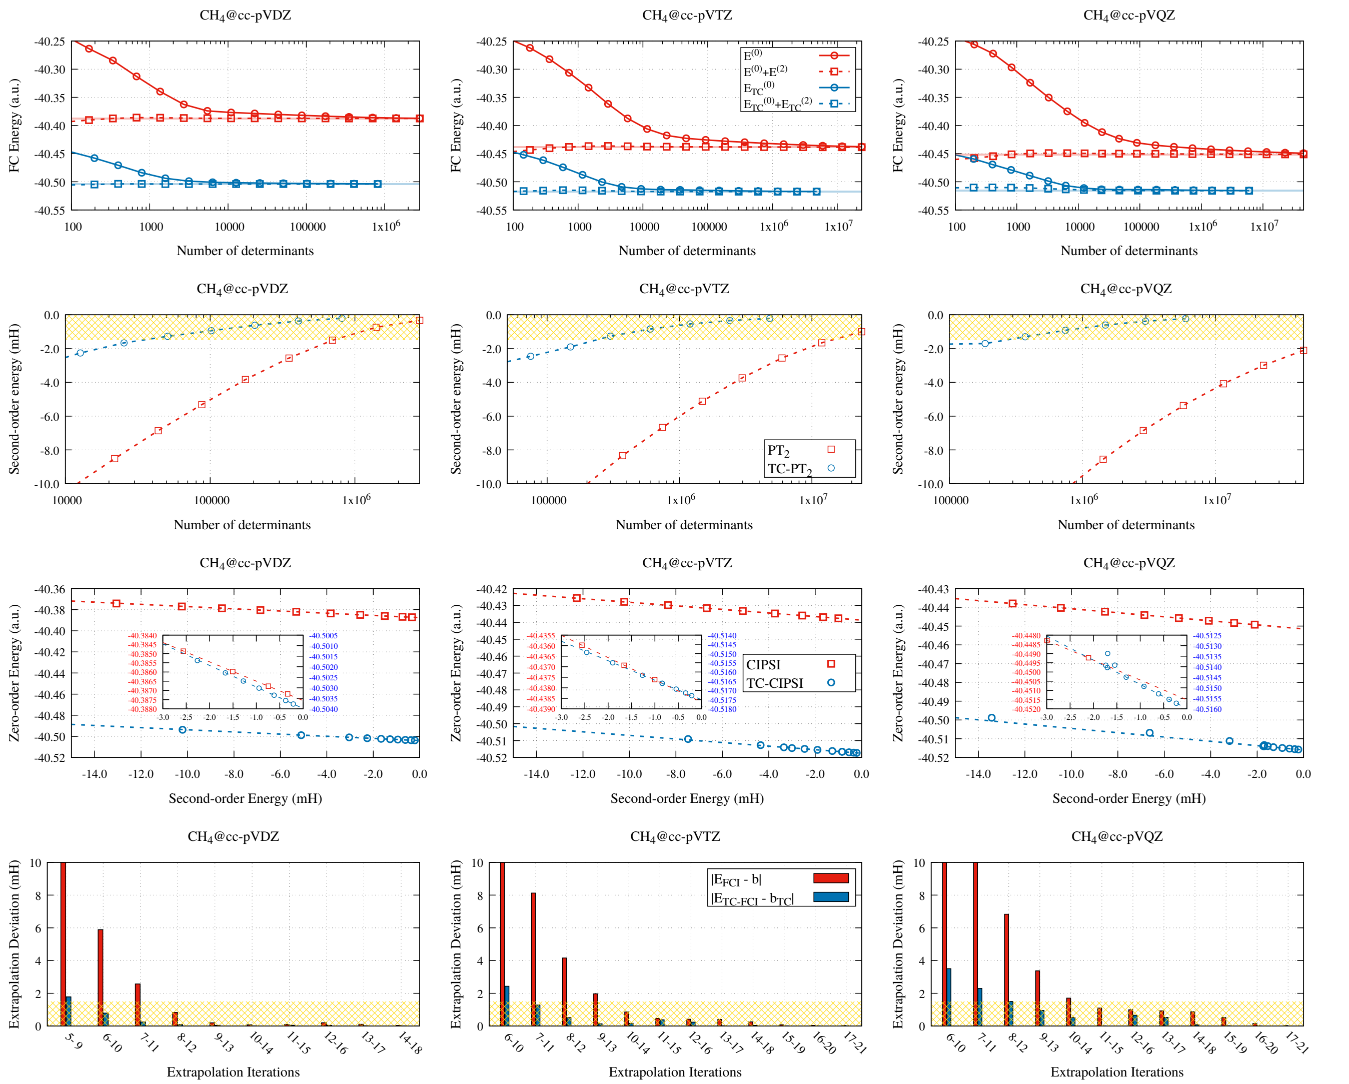


FIG. 5. Convergence analysis of frozen-core calculations for $CH_4$ molecule using different basis sets. Each row represents a different aspect of the convergence analysis, with three panels corresponding to different basis sets: cc-pVDZ (left), cc-pVTZ (middle), and cc-pVQZ (right).

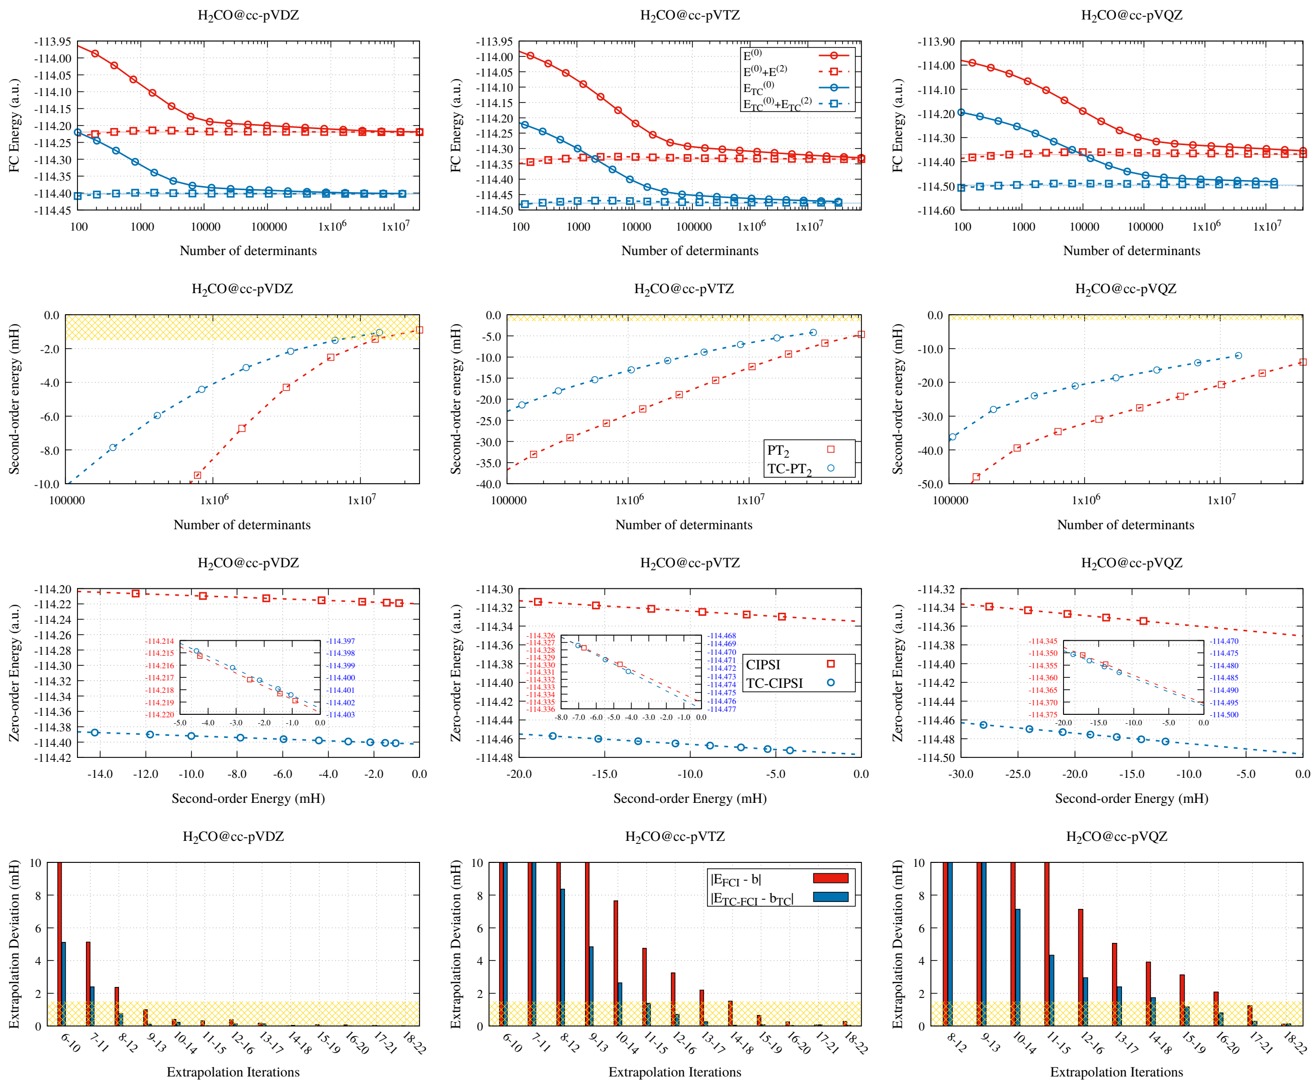


FIG. 6. Convergence analysis of frozen-core calculations for $H_2CO$ molecule using different basis sets. Each row represents a different aspect of the convergence analysis, with three panels corresponding to different basis sets: cc-pVDZ (left), cc-pVTZ (middle), and cc-pVQZ (right).

TABLE I. Number of determinants required in CIPSI and TC-CIPSI (and their corresponding ratio) to achieve a given second-order perturbative energies (PT2) of 1.5 m$E_\mathrm{h}$, 3.0 m$E_\mathrm{h}$, 7.5 m$E_\mathrm{h}$, 15.0 m$E_\mathrm{h}$, and 30.0 m$E_\mathrm{h}$ for $Li_2$, $H_2O$, $NH_3$, $CH_4$, and $H_2CO$ across different basis sets.

| | cc-pVDZ | | | cc-pVTZ | | | cc-pVQZ | | |
|---|---|---|---|---|---|---|---|---|---|
| **$Li_2$** | | | | | | | | | |
| PT2 | CIPSI | TC-CIPSI | ratio | CIPSI | TC-CIPSI | ratio | CIPSI | TC-CIPSI | ratio |
| 1.5 m$E_\mathrm{h}$ | 41 | 59 | 0.7 | 2 317 | 684 | 3.4 | 14 939 | 2 854 | 5.2 |
| 3.0 m$E_\mathrm{h}$ | 32 | 39 | 0.8 | 873 | 255 | 3.4 | 5 003 | 1 069 | 4.7 |
| 7.5 m$E_\mathrm{h}$ | 17 | 20 | 0.8 | 181 | 76 | 2.4 | 1 106 | 218 | 5.1 |
| 15.0 m$E_\mathrm{h}$ | 8 | 8 | 1.1 | 64 | 28 | 2.3 | 286 | 60 | 4.8 |
| 30.0 m$E_\mathrm{h}$ | 2 | 1 | 1.7 | 18 | 8 | 2.2 | 64 | 12 | 5.2 |
| **$Be_2$** | | | | | | | | | |
| PT2 | CIPSI | TC-CIPSI | ratio | CIPSI | TC-CIPSI | ratio | CIPSI | TC-CIPSI | ratio |
| 1.5 m$E_\mathrm{h}$ | 2 759 | 1 423 | 1.9 | 48 222 | 10 994 | 4.4 | 430 813 | 44 673 | 9.6 |
| 3.0 m$E_\mathrm{h}$ | 1 357 | 734 | 1.9 | 13 646 | 4 274 | 3.2 | 119 850 | 15 138 | 7.9 |
| 7.5 m$E_\mathrm{h}$ | 431 | 256 | 1.7 | 3 172 | 1 069 | 3.0 | 18 250 | 2 966 | 6.2 |
| 15.0 m$E_\mathrm{h}$ | 194 | 133 | 1.5 | 871 | 329 | 2.6 | 4 677 | 792 | 5.9 |
| 30.0 m$E_\mathrm{h}$ | 86 | 58 | 1.5 | 228 | 107 | 2.1 | 852 | 204 | 4.2 |
| **$H_2O$** | | | | | | | | | |
| PT2 | CIPSI | TC-CIPSI | ratio | CIPSI | TC-CIPSI | ratio | CIPSI | TC-CIPSI | ratio |
| 1.5 m$E_\mathrm{h}$ | 96 883 | 12 195 | 8.0 | 3 105 054 | 148 821 | 20.9 | 23 609 437 | 781 281 | 30.2 |
| 3.0 m$E_\mathrm{h}$ | 41 175 | 2 691 | 15.3 | 1 175 264 | 25 262 | 46.5 | 8 011 050 | 182 028 | 44.0 |
| 7.5 m$E_\mathrm{h}$ | 5 892 | 1 235 | 4.8 | 190 598 | 6 008 | 31.7 | 1 143 925 | 20 226 | 56.6 |
| 15.0 m$E_\mathrm{h}$ | 1 427 | 756 | 1.9 | 21 369 | 2 849 | 7.5 | 115 280 | 7 918 | 14.6 |
| 30.0 m$E_\mathrm{h}$ | 927 | 415 | 2.2 | 7 216 | 1 161 | 6.2 | 24 938 | 3 087 | 8.1 |
| **$NH_3$** | | | | | | | | | |
| PT2 | CIPSI | TC-CIPSI | ratio | CIPSI | TC-CIPSI | ratio | CIPSI | TC-CIPSI | ratio |
| 1.5 m$E_\mathrm{h}$ | 1 031 535 | 88 913 | 11.6 | 23 512 245 | 1 388 400 | 16.9 | – | 3 473 148 | – |
| 3.0 m$E_\mathrm{h}$ | 250 276 | 14 731 | 17.0 | 8 038 195 | 284 942 | 28.2 | 41 831 306 | 676 984 | 61.8 |
| 7.5 m$E_\mathrm{h}$ | 25 268 | 3 231 | 7.8 | 1 028 788 | 24 392 | 42.2 | 4 486 257 | 42 929 | 104.5 |
| 15.0 m$E_\mathrm{h}$ | 5 671 | 1 747 | 3.3 | 91 807 | 9 884 | 9.3 | 405 463 | 14 610 | 27.8 |
| 30.0 m$E_\mathrm{h}$ | 2 864 | 816 | 3.5 | 22 970 | 3 712 | 6.2 | 72 182 | 5 527 | 13.1 |
| **$CH_4$** | | | | | | | | | |
| PT2 | CIPSI | TC-CIPSI | ratio | CIPSI | TC-CIPSI | ratio | CIPSI | TC-CIPSI | ratio |
| 1.5 m$E_\mathrm{h}$ | 703 021 | 34 036 | 20.7 | 14 057 992 | 232 586 | 60.4 | – | 264 076 | – |
| 3.0 m$E_\mathrm{h}$ | 276 102 | 6 559 | 42.1 | 4 587 477 | 37 703 | 121.7 | 22 819 072 | 13 354 | 1 708.7 |
| 7.5 m$E_\mathrm{h}$ | 33 491 | 2 291 | 14.6 | 526 121 | 4 677 | 112.5 | 2 201 275 | 5 734 | 383.9 |
| 15.0 m$E_\mathrm{h}$ | 4 831 | 1 126 | 4.3 | 46 701 | 2 419 | 19.3 | 191 898 | 2 850 | 67.3 |
| 30.0 m$E_\mathrm{h}$ | 2 273 | 462 | 4.9 | 12 573 | 1 025 | 12.3 | 38 097 | 892 | 42.7 |
| **$H_2CO$** | | | | | | | | | |
| PT2 | CIPSI | TC-CIPSI | ratio | CIPSI | TC-CIPSI | ratio | CIPSI | TC-CIPSI | ratio |
| 1.5 m$E_\mathrm{h}$ | 12 105 126 | 6 824 210 | 1.8 | – | – | – | – | – | – |
| 3.0 m$E_\mathrm{h}$ | 5 208 936 | 1 841 563 | 2.8 | – | – | – | – | – | – |
| 7.5 m$E_\mathrm{h}$ | 1 295 299 | 239 345 | 5.4 | 34 155 513 | 7 104 030 | 4.8 | – | – | – |
| 15.0 m$E_\mathrm{h}$ | 216 760 | 22 260 | 9.7 | 5 900 797 | 593 392 | 9.9 | 32 990 562 | 5 253 967 | 6.3 |
| 30.0 m$E_\mathrm{h}$ | 11 656 | 4 520 | 2.6 | 281 404 | 42 124 | 6.7 | 1 531 565 | 179 956 | 8.5 |

TABLE II. Number of determinants required in CIPSI and TC-CIPSI (and their corresponding ratio) to converge to chemical accuracy the extrapolated estimate of the total energy of $Li_2$, $Be_2$, $H_2O$, $NH_3$, $CH_4$, and $H_2CO$ across different basis sets.

| | | cc-pVDZ | cc-pVTZ | cc-pVQZ |
|---|---|---|---|---|
| | CIPSI | 42 | 44 | 71 |
| $Li_2$ | TC-CIPSI | 40 | 42 | 43 |
| | ratio | 1.1 | 1.1 | 1.7 |
| | CIPSI | 287 | 957 | 1 843 |
| $Be_2$ | TC-CIPSI | 256 | 239 | 228 |
| | ratio | 1.1 | 4.0 | 8.1 |
| | CIPSI | 2 834 | 9 821 | 22 248 |
| $H_2O$ | TC-CIPSI | 729 | 3 085 | 3 063 |
| | ratio | 3.9 | 3.2 | 7.3 |
| | CIPSI | 3 102 | 26 045 | 30 404 |
| $NH_3$ | TC-CIPSI | 495 | 6 564 | 5 733 |
| | ratio | 6.3 | 4.0 | 5.3 |
| | CIPSI | 5 452 | 11 608 | 24 244 |
| $CH_4$ | TC-CIPSI | 791 | 2 343 | 3 235 |
| | ratio | 6.9 | 5.0 | 7.5 |
| | CIPSI | 12 272 | 82 615 | 159 259 |
| $H_2CO$ | TC-CIPSI | 13 108 | 33 148 | 53 268 |
| | ratio | 0.9 | 2.5 | 3.0 |

TABLE III. Total energies (in $E_\mathrm{h}$) and ionization potentials (in eV) obtained from FCI and TC-FCI calculations, with or without frozen-core (FC) approximation, in the cc-pVXZ basis sets for the neutral and ionized atoms from $Z = 2$ to $Z = 10$.

| | He | | $He^+$ | | IP (eV) | |
|---|---|---|---|---|---|---|
| | FCI | TC-FCI | FCI | TC-FCI | FCI | TC-FCI |
| cc-pVDZ | -2.887 6 | -2.897 5 | -1.993 6 | -1.993 6 | 24.33 | 24.60 |
| cc-pVTZ | -2.900 2 | -2.903 3 | -1.998 9 | -1.998 9 | 24.53 | 24.61 |
| cc-pVQZ | -2.902 4 | -2.903 7 | -1.999 8 | -1.999 8 | 24.56 | 24.59 |
| cc-pV5Z | -2.903 2 | | -1.999 9 | | 24.58 | |
| Ref. | -2.903 7 | | | | 24.59 | |

| | Li | | $Li^+$ | | IP (eV) | |
|---|---|---|---|---|---|---|
| | FCI | TC-FCI | FCI | TC-FCI | FCI | TC-FCI |
| cc-pVDZ | -7.432 6 | -7.477 1 | -7.236 2 | -7.288 6 | 5.35 | 5.13 |
| cc-pVTZ | -7.446 1 | -7.478 1 | -7.249 4 | -7.279 5 | 5.35 | 5.40 |
| cc-pVQZ | -7.449 8 | -7.478 5 | -7.252 5 | -7.280 0 | 5.37 | 5.40 |
| cc-pV5Z | -7.456 3 | | -7.258 6 | | 5.38 | |
| Ref. | -7.478 1 | | | | 5.39 | |

| | Be | | $Be^+$ | | IP (eV) | |
|---|---|---|---|---|---|---|
| | FCI | TC-FCI | FCI | TC-FCI | FCI | TC-FCI |
| cc-pVDZ | -14.617 4 | -14.668 1 | -14.276 0 | -14.326 7 | 9.29 | 9.29 |
| cc-pVTZ | -14.623 8 | -14.668 1 | -14.282 6 | -14.325 4 | 9.29 | 9.32 |
| cc-pVQZ | -14.640 2 | -14.667 6 | -14.298 3 | -14.324 8 | 9.30 | 9.33 |
| cc-pV5Z | -14.646 4 | | -14.304 2 | | 9.31 | |
| Ref. | -14.667 4 | | | | 9.32 | |

| | B | | | $B^+$ | | | IP (eV) | | |
|---|---|---|---|---|---|---|---|---|---|
| | FCI (FC) | TC-FCI (FC) | TC-FCI | FCI (FC) | TC-FCI (FC) | TC-FCI | FCI (FC) | TC-FCI (FC) | TC-FCI |
| cc-pVDZ | -24.589 8 | -24.645 3 | -24.645 1 | -24.293 1 | -24.345 8 | -24.345 7 | 8.07 | 8.15 | 8.15 |
| cc-pVTZ | -24.598 6 | -24.648 0 | -24.649 9 | -24.296 5 | -24.342 6 | -24.344 4 | 8.22 | 8.31 | 8.31 |
| cc-pVQZ | -24.601 3 | -24.647 5 | -24.652 7 | -24.298 4 | -24.342 5 | -24.347 9 | 8.24 | 8.30 | 8.30 |
| cc-pV5Z | -24.602 0 | | | -24.298 7 | | | 8.25 | | |
| Ref. | | -24.653 9 | | | | | | 8.30 | |

| | C | | | $C^+$ | | | IP (eV) | | |
|---|---|---|---|---|---|---|---|---|---|
| | FCI (FC) | TC-FCI (FC) | TC-FCI | FCI (FC) | TC-FCI (FC) | TC-FCI | FCI (FC) | TC-FCI (FC) | TC-FCI |
| cc-pVDZ | -37.760 8 | -37.827 5 | -37.827 5 | -37.357 2 | -37.420 2 | -37.420 2 | 10.98 | 11.08 | 11.08 |
| cc-pVTZ | -37.781 3 | -37.836 4 | -37.839 0 | -37.370 8 | -37.422 0 | -37.424 6 | 11.17 | 11.27 | 11.28 |
| cc-pVQZ | -37.787 1 | -37.837 1 | -37.844 3 | -37.375 2 | -37.422 9 | -37.430 3 | 11.21 | 11.27 | 11.27 |
| cc-pV5Z | -37.788 7 | | | -37.376 4 | | | 11.22 | | |
| Ref. | | -37.845 0 | | | | | | 11.26 | |

| | N | | | $N^+$ | | | IP (eV) | | |
|---|---|---|---|---|---|---|---|---|---|
| | FCI (FC) | TC-FCI (FC) | TC-FCI | FCI (FC) | TC-FCI (FC) | TC-FCI | FCI (FC) | TC-FCI (FC) | TC-FCI |
| cc-pVDZ | -54.478 7 | -54.556 9 | -54.556 9 | -53.957 3 | -54.030 3 | -54.030 3 | 14.19 | 14.33 | 14.33 |
| cc-pVTZ | -54.515 0 | -54.576 3 | -54.579 5 | -53.984 7 | -54.041 4 | -54.044 5 | 14.43 | 14.56 | 14.56 |
| cc-pVQZ | -54.525 1 | -54.579 0 | -54.588 0 | -53.992 8 | -54.044 1 | -54.053 1 | 14.49 | 14.56 | 14.56 |
| cc-pV5Z | -54.528 2 | | | -53.995 2 | | | 14.51 | | |
| Ref. | | -54.589 2 | | | | | | 14.53 | |

| | O | | | $O^+$ | | | IP (eV) | | |
|---|---|---|---|---|---|---|---|---|---|
| | FCI (FC) | TC-FCI (FC) | TC-FCI | FCI (FC) | TC-FCI (FC) | TC-FCI | FCI (FC) | TC-FCI (FC) | TC-FCI |
| cc-pVDZ | -74.910 2 | -75.016 5 | -75.016 3 | -74.437 9 | -74.533 8 | -74.533 8 | 12.85 | 13.13 | 13.13 |
| cc-pVTZ | -74.974 2 | -75.049 9 | -75.052 7 | -74.484 8 | -74.550 9 | -74.553 9 | 13.32 | 13.58 | 13.58 |
| cc-pVQZ | -74.993 9 | -75.056 6 | -75.065 8 | -74.498 4 | -74.555 9 | -74.565 3 | 13.48 | 13.63 | 13.62 |
| cc-pV5Z | -75.000 4 | | | -74.502 6 | | | 13.55 | | |
| Ref. | | -75.067 3 | | | | | | 13.62 | |

| | F | | | $F^+$ | | | IP (eV) | | |
|---|---|---|---|---|---|---|---|---|---|
| | FCI (FC) | TC-FCI (FC) | TC-FCI | FCI (FC) | TC-FCI (FC) | TC-FCI | FCI (FC) | TC-FCI (FC) | TC-FCI |
| cc-pVDZ | -99.527 8 | -99.658 9 | -99.658 6 | -98.913 7 | -99.031 0 | -99.030 8 | 16.71 | 17.09 | 17.08 |
| cc-pVTZ | -99.620 6 | -99.711 0 | -99.713 9 | -98.990 9 | -99.069 7 | -99.072 7 | 17.13 | 17.45 | 17.45 |
| cc-pVQZ | -99.650 5 | -99.723 0 | -99.732 9 | -99.014 6 | -99.080 4 | -99.090 4 | 17.30 | 17.49 | 17.48 |
| cc-pV5Z | -99.660 8 | | | -99.022 6 | | | 17.37 | | |
| Ref. | | -99.733 9 | | | | | | 17.42 | |

| | Ne | | | $Ne^+$ | | | IP (eV) | | |
|---|---|---|---|---|---|---|---|---|---|
| | FCI (FC) | TC-FCI (FC) | TC-FCI | FCI (FC) | TC-FCI (FC) | TC-FCI | FCI (FC) | TC-FCI (FC) | TC-FCI |
| cc-pVDZ | -128.679 0 | -128.837 9 | -128.837 5 | -127.911 2 | -128.058 0 | -128.057 7 | 20.89 | 21.22 | 21.22 |
| cc-pVTZ | -128.802 5 | -128.907 2 | -128.909 9 | -128.019 8 | -128.112 8 | -128.115 6 | 21.30 | 21.62 | 21.62 |
| cc-pVQZ | -128.843 8 | -128.926 0 | -128.936 0 | -128.054 6 | -128.129 7 | -128.139 7 | 21.47 | 21.67 | 21.67 |
| cc-pV5Z | -128.858 4 | | | -128.066 8 | | | 21.54 | | |
| Ref. | | -128.937 6 | | | | | | 21.56 | |

TABLE IV. Total energies (in $E_\mathrm{h}$) and ionization potentials (in eV) obtained from FCI and TC-FCI calculations, with or without frozen-core (FC) approximation, in the cc-pVXZ basis sets for the neutral and ionized molecules ($Li_2$, $Be_2$, $H_2O$, $NH_3$, $CH_4$, and $H_2CO$).

| | $Li_2$ | | $Li_2^+$ | | IP (eV) | |
|---|---|---|---|---|---|---|
| | FCI | TC-FCI | FCI | TC-FCI | FCI | TC-FCI |
| cc-pVDZ | -14.901 4 | -14.977 6 | -14.710 6 | -14.787 3 | 5.19 | 5.18 |
| cc-pVTZ | -14.931 3 | -14.988 8 | -14.739 4 | -14.795 6 | 5.22 | 5.26 |
| cc-pVQZ | -14.941 2 | -14.991 8 | -14.748 6 | -14.798 1 | 5.24 | 5.27 |
| cc-pV5Z | -14.954 2 | | -14.761 4 | | 5.25 | |
| extrap | | | | | 5.25 | |

| | $Be_2$ | | $Be_2^+$ | | IP (eV) | |
|---|---|---|---|---|---|---|
| | FCI | TC-FCI | FCI | TC-FCI | FCI | TC-FCI |
| cc-pVDZ | -29.235 4 | -29.324 5 | -28.962 1 | -29.049 2 | 7.44 | 7.47 |
| cc-pVTZ | -29.254 7 | -29.326 8 | -28.980 8 | -29.051 3 | 7.45 | 7.50 |
| cc-pVQZ | -29.285 0 | -29.339 5 | -29.010 5 | -29.063 9 | 7.47 | 7.50 |
| cc-pV5Z | -29.298 1 | | -29.023 3 | | 7.48 | |
| extrap | | | | | 7.49 | |

| | $H_2O$ | | | $H_2O^+$ | | | IP (eV) | | |
|---|---|---|---|---|---|---|---|---|---|
| | FCI (FC) | TC-FCI (FC) | TC-FCI | FCI (FC) | TC-FCI (FC) | TC-FCI | FCI (FC) | TC-FCI (FC) | TC-FCI |
| cc-pVDZ | -76.241 7 | -76.378 2 | -76.377 5 | -75.802 3 | -75.921 2 | -75.920 7 | 11.96 | 12.44 | 12.43 |
| cc-pVTZ | -76.332 6 | -76.420 4 | -76.423 4 | -75.873 8 | -75.953 1 | -75.956 2 | 12.49 | 12.72 | 12.71 |
| cc-pVQZ | -76.360 2 | -76.428 0 | -76.436 7 | -75.894 9 | -75.959 0 | -75.967 8 | 12.66 | 12.76 | 12.76 |
| cc-pV5Z | -76.369 5 | | | -75.901 5 | | | 12.73 | | |
| extrap | | | | | | | 12.80 | | |

| | $NH_3$ | | | $NH_3^+$ | | | IP (eV) | | |
|---|---|---|---|---|---|---|---|---|---|
| | FCI (FC) | TC-FCI (FC) | TC-FCI | FCI (FC) | TC-FCI (FC) | TC-FCI | FCI (FC) | TC-FCI (FC) | TC-FCI |
| cc-pVDZ | -56.402 6 | -56.516 5 | -56.516 2 | -56.023 2 | -56.124 1 | -56.123 9 | 10.32 | 10.68 | 10.68 |
| cc-pVTZ | -56.473 7 | -56.552 2 | -56.556 6 | -56.078 2 | -56.151 1 | -56.155 5 | 10.76 | 10.92 | 10.91 |
| cc-pVQZ | -56.493 6 | -56.557 1 | -56.565 5 | -56.093 3 | -56.154 3 | -56.162 8 | 10.89 | 10.96 | 10.96 |
| cc-pV5Z | -56.500 0 | | | -56.097 6 | | | 10.95 | | |
| extrap | | | | | | | 11.00 | | |

| | $CH_4$ | | | $CH_4^+$ | | | IP (eV) | | |
|---|---|---|---|---|---|---|---|---|---|
| | FCI (FC) | TC-FCI (FC) | TC-FCI | FCI (FC) | TC-FCI (FC) | TC-FCI | FCI (FC) | TC-FCI (FC) | TC-FCI |
| cc-pVDZ | -40.387 5 | -40.504 0 | -40.503 1 | -39.865 8 | -39.974 0 | -39.974 0 | 14.20 | 14.42 | 14.40 |
| cc-pVTZ | -40.438 7 | -40.517 5 | -40.521 1 | -39.911 0 | -39.985 9 | -39.989 4 | 14.36 | 14.47 | 14.47 |
| cc-pVQZ | -40.451 5 | -40.516 0 | -40.520 7 | -39.922 3 | -39.985 4 | -39.990 0 | 14.40 | 14.44 | 14.44 |
| cc-pV5Z | -40.455 2 | | | -39.925 5 | | | 14.41 | | |
| extrap | | | | | | | 14.43 | | |

| | $H_2CO$ | | | $H_2CO^+$ | | | IP (eV) | | |
|---|---|---|---|---|---|---|---|---|---|
| | FCI (FC) | TC-FCI (FC) | TC-FCI | FCI (FC) | TC-FCI (FC) | TC-FCI | FCI (FC) | TC-FCI (FC) | TC-FCI |
| cc-pVDZ | -114.219 9 | -114.402 5 | -114.401 2 | -113.836 1 | -114.007 1 | -114.005 9 | 10.44 | 10.76 | 10.76 |
| cc-pVTZ | -114.335 1 | -114.477 0 | -114.483 5 | -113.938 4 | -114.074 5 | -114.081 0 | 10.80 | 10.95 | 10.95 |
| cc-pVQZ | -114.370 6 | -114.496 5 | -114.509 7 | -113.969 3 | -114.092 9 | -114.106 3 | 10.92 | 10.98 | 10.98 |
| cc-pV5Z | -114.382 0 | | | -113.979 5 | | | 10.95 | | |
| extrap | | | | | | | 11.00 | | |

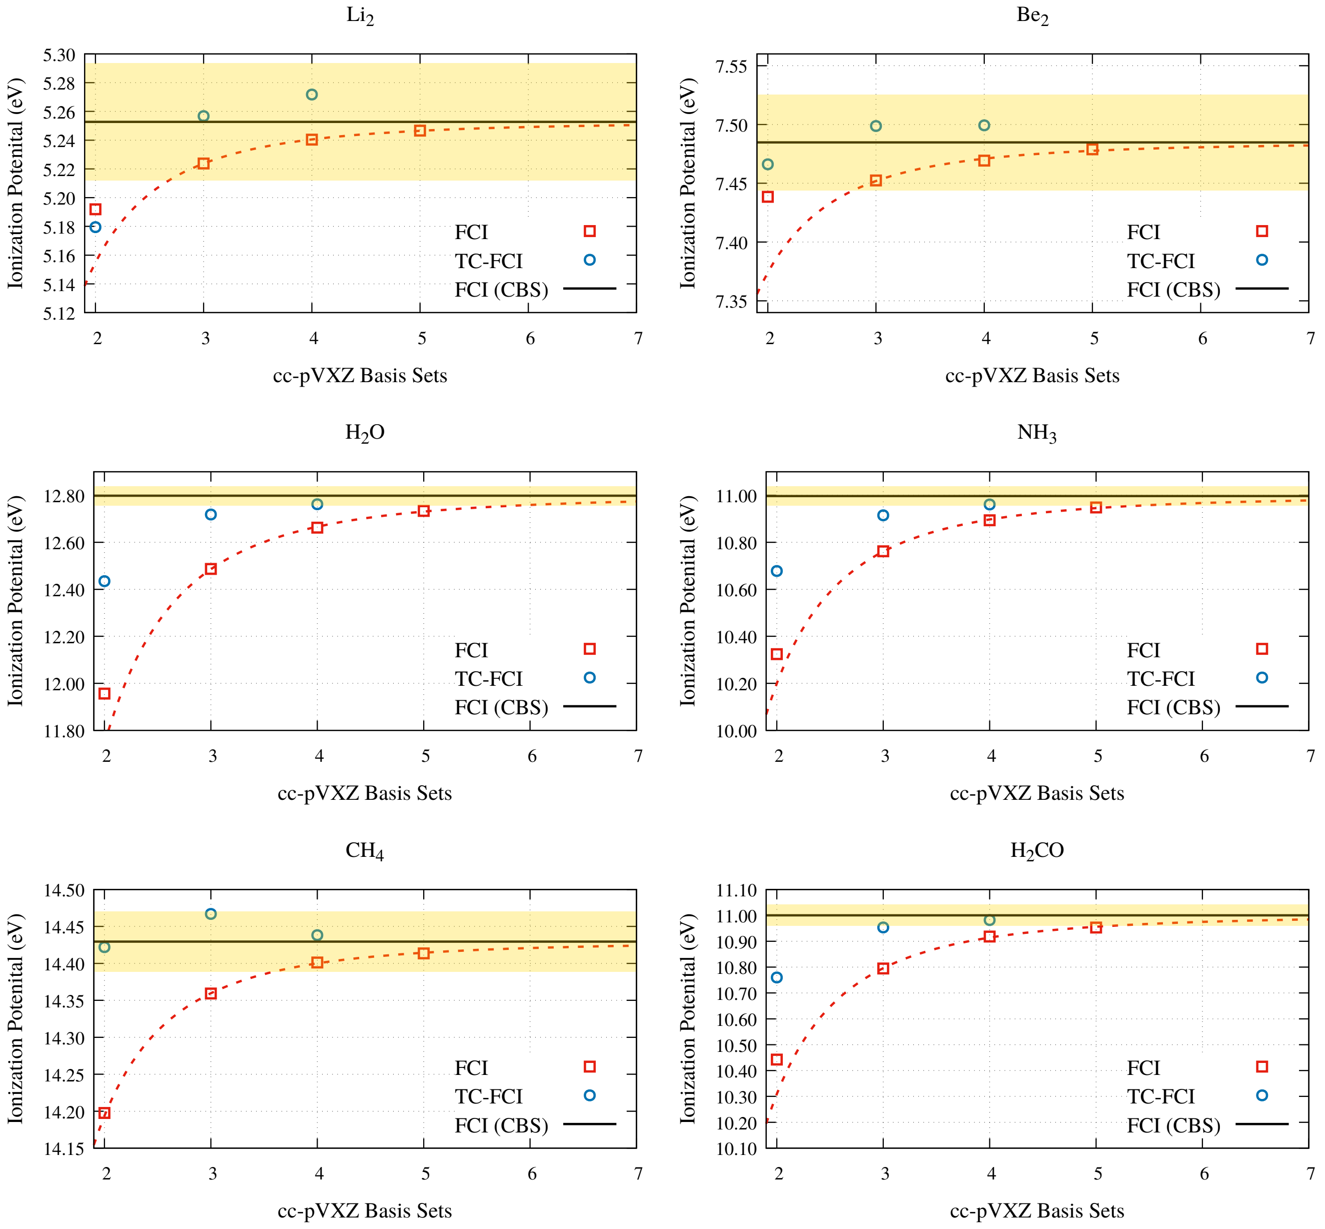


FIG. 7. Ionization potentials (in eV) of $Li_2$, $Be_2$, $H_2O$, $NH_3$, $CH_4$ and $H_2CO$ computed at the FCI and TC-FCI levels with the cc-pVXZ family of basis sets. To produce CBS estimates (black solid lines), we have extrapolated the IPs obtained at the FCI level using an inverse cubic parametrization, across the cc-pVXZ basis sets (where X = T, Q, and 5). The shaded yellow region corresponds to $1.5\,\mathrm{m}E_\mathrm{h}$ accuracy.

## REFERENCES

[1]N. C. H. Peter T. A. Galek and W. A. L. Jr, Mol. Phys. **104**, 3069 (2006).
[2]A. Ammar, E. Giner, and A. Scemama, J. Chem. Theory Comput. **18**, 5325 (2022).
